# Supplementary material for: Rheology of Thickly-Coated Granular-Fluid Systems
Source: arXiv:1812.07083 source file (2018-12-17)
Supplement: Supplementary file 1 [file Supplemental_Materials_1.pdf]

# Rheology of Thickly-Coated Granular-Fluid Systems
# Supplemental Material I

Teng Man, Qingfeng Feng, and Kimberly Hill
(Dated: December 13, 2018)

## INTER-PARTICLE CONTACT LAW

In our simulations, both the normal and tangential contact forces are calculated based on Hertz-Mindlin contact theories [1] and damping components based on the derivation outlined by Tsuji et al. [2]. In this model, the tangential contact force also follows the Coulomb friction law, where the tangential contact forces cannot exceed $\mu_p F_c$.

$$F_c^{\mathrm{ij,n}} = -k_n \delta_n^{1.5} - \eta_n \delta_n^{0.25} \dot{\delta}_n \tag{1a}$$

$$F_c^{\mathrm{ij,t}} = \min\big( - \mathrm{k_t} \delta_\mathrm{n}^{0.5} \delta_\mathrm{t} - \eta_\mathrm{t} \delta_\mathrm{n}^{0.25} \dot{\delta}_\mathrm{t}, \mu_\mathrm{p} F_c^{\mathrm{ij,n}} \big) \tag{1b}$$

where $F_c^{\mathrm{ij,n}}$ and $F_c^{\mathrm{ij,t}}$ are normal and tangential contact forces acting on particle $i$ from particle $j$. $\delta_n$ is the overlap between particles in normal direction in DEM simulation, which is given by $\delta_n = R_i + R_j - |\vec{r}_i - \vec{r}_j|$, where $R_i$ and $R_j$ are particle radii, and $\vec{r}_i$ and $\vec{r}_j$ are position vectors of two particles. $\delta_t$ is the corresponding tangential deformation at the contact point between two particles, and $\mu_p$ is the coefficient of friction. The coefficients in the contact model are related to material properties of two contacting particles presented in Table I. In this simulation, the particle density is 2650 kg/m$^3$, elastic modulus is 29 GPa, and the Poisson's ratio is 0.20. The material properties are based on those of granite spheres. In order to calculate the dissipative term, the coefficient of restitution is set to be around 0.20. Usually, in studies related to granular materials, the particles are relatively smooth and elastic. However, in this study, we chose a relatively small number for the coefficient of restitution to capture a more representative collisional behavior of granite sand particles whose collisions are less elastic. According to Foerster, et al. [3], the coefficient of friction between particles, $\mu_p$, is set to be 0.10.

TABLE I. Relationships for calculating the stiffnesses and damping coefficients in Eq. 1(a) and (b)

| Variables | Equations |
|---|---|
| $k_n$ | $(4/3)\sqrt{R_\mathrm{eff}} E_\mathrm{eff}$ |
| $k_t$ | $8\sqrt{R_\mathrm{eff}} G_\mathrm{eff}$ |
| $\eta_n$ | $\alpha_o \sqrt{m_\mathrm{eff} k_n}$ |
| $\eta_t$ | $\alpha_o \sqrt{m_\mathrm{eff} k_t}$ |
| $R_\mathrm{eff}$ | $(1/R_i + 1/R_j)^{-1}$ |
| $E_\mathrm{eff}$ | $((1-\nu_i^2)/E_i + (1-\nu_j^2)/E_j)^{-1}$ |
| $G_\mathrm{eff}$ | $(2(1+\nu_i)(2-\nu_i)/E_i + 2(1+\nu_j)(2-\nu_j)/E_j)^{-1}$ |
| $m_\mathrm{eff}$ | $(1/m_i + 1/m_j)^{-1}$ |

$\alpha_o = 0.9$ is calculated based on the relationship between $\alpha_o$ and $e$ proposed by Tsuji et al. [2]. $E_i$ and $E_j$ are elastic moduli, $\nu_i$ and $\nu_j$ are Poisson's ratios, and $m_i$ and $m_j$ are masses of contacting particles $i$ and $j$.

## LUBRICATION EFFECT

To model the influence of properties of a fluid that thickly coats all particles, we use a lubrication model by Pitois, et al.[4] and Goldman et al. [5] as in Refs. [6, 7]. As summarized in the main text, the forces due to a thick coating between two particles, normal and tangential to their closest surface points can be written using following equations:

$$F_v^{\mathrm{ij,n}} = 6\pi\eta R_\mathrm{eff}^2 G_f^2 \frac{v_n^\mathrm{rel}}{\delta_g} \tag{2a}$$

$$F_v^{\mathrm{ij,t}} = 6\pi\eta R_\mathrm{eff} v_t^\mathrm{rel} \big[\frac{8}{15} \mathrm{ln}(\mathrm{R_{eff}}/\delta_\mathrm{g}) + 0.9588\big] \tag{2b}$$

where $F_v^{\mathrm{ij,n}}$ and $F_v^{\mathrm{ij,t}}$ are normal and tangential lubrication forces between particle $i$ and particle $j$. $R_\mathrm{eff}$ is the effective radius calculated based on the radius of two contacting particles. $v_n^\mathrm{rel}$ and $v_t^\mathrm{rel}$ are relative normal velocity and relative tangential velocity, respectively. $\eta$ is the fluid viscosity, and $\delta_g$ is the gap between the nearest surface of two particles. $G_f$ is a coefficient considering the effective volume which have lubrication effect to make sure that the effect of lubrication will be decreased as we increase the gap between adjacent particles.

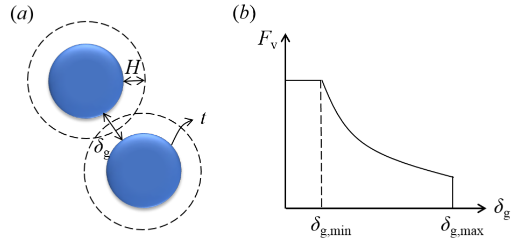


FIG. 1. Sketches for considering particle roughness, $t$, and maximum lubrication length, $H$.

As we mention in the main text, we use two regularizing length scales for this viscous force: (1) $\delta_{\mathrm{g,min}} \sim \langle d \rangle/10 \approx 2t$ can be thought of as twice a typical particle roughness length scale, $t$, and (2) $\delta_{\mathrm{g,max}} \sim \langle d \rangle \approx 2H$

(twice the maximum lubrication length scale, $H$). In this study, we consider thick coating on the surface of particles, thus, when the distance between two particle is too large, the lubrication effect should be negligible. We choose average particle diameter as the maximum lubrication length scale to restrict the lubrication forces to those between two particles only when they are reasonably close. For instance, when the distance of two particles is larger than a particle diameter, another particle may get into the gap between two particles, thus, the lubrication effect should not be considered. FIG. 1 shows the schematic relationship between lubrication forces, $F_v^{\mathrm{ij,n}}$ or $F_v^{\mathrm{ij,t}}$, and particle gap, $\delta$, keeping the relative particle velocities constant. $G_f$ is calculated using the following equation:

$$G_f = 1 - \frac{1}{\sqrt{1 + \frac{\bar{V}}{\pi R_{\mathrm{eff}} \delta_g^2}}} \tag{3}$$

where $\bar{V}$ is the effective lubrication volume, and $\bar{V} = [\delta_{\mathrm{g,max}}/(1 + 0.5\theta_c)]^3$. Here, we consider $\delta_{\mathrm{g,max}}$ as a rupture distance when no lubrication effects exist between two adjacent particles. $\theta_c$ is contact angle of the interstitial fluid and associated to the surface energy of the interstitial fluid. In this simulation, we set $\theta_c$ to be equal to 0.5. In this simulation, $G_f$ approximately varies from 0.9 to 0.22. In a system where the granular material is fully saturated with fluid, $G_f = 1$. To consider the importance of this limited fluid volume effect, we also simulated the simple shear test with $G_f = 1.0$. The results are shown in FIG. 2. The results show that the effect of using $G_f < 1$ in the range relevant to our problem is essentially negligible.

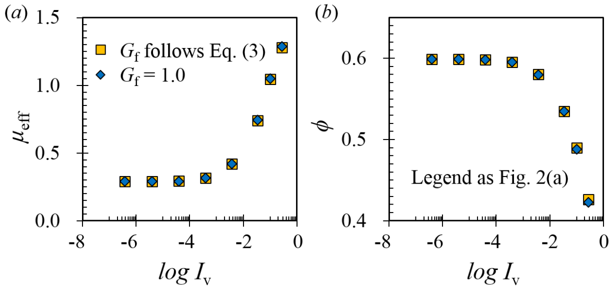


FIG. 2. Comparison between simulation results when we take $G_f$ = Eq. 3 (■) and that when we take $G_f = 1.0$ (◆).

## SCALING OF GRANULAR TEMPERATURE

In FIG. 3(d) of the main text, we plotted a measured granular temperature, $T_g$, i.e., granular temperature per unit volume, also with units of stress. We showed that for $\phi \gtrsim 0.51$, $T_g$ scales with the proximity of solid fraction, to its effective maximum, $\phi_m - \phi$. We compare these results to predictions of Bagnold [8] according to his theory relating stresses to rates of average interparticle collisions, distances, etc., based on imposed conditions. With a relatively simple collisional model, Bagnold derived a form for a normalized dispersive stresses that scales with $\lambda \equiv 1/[(\phi_0/\phi)^{1/3} - 1]$. His data suggest that a normalized form of $\tau_c$ scales with $\lambda^2$ when the effects of grain inertia dominate, and that the normalized dispersive stresses scale with $\lambda^{1.5}$ when the effects of fluid viscosity dominate. Here $\phi_0$ is the maximum possible static volume fraction of granular material and is equal to 0.74. In FIG. 3(a), we plotted the relationship between $T_g \rho_p d^2/(\lambda \eta^2)$ and Bagnold number $Ba = \lambda^{0.5} \rho_p d^2 \dot{\gamma}/\eta$. Similar to the results obtained by Bagnold, the normalized granular temperature (kinetic stress) roughly scales with the squared Bagnold number, except when $Ba$ is small and $J$ is large (● in FIG. 3(a)), the data are more scattered. We then plotted the relationship between solid fraction and the normalized granular temperature in FIG. 2(b) (In FIG. 2(b), $\tilde{T}_g = T_g/(\rho_p \dot{\gamma}^2 d^2)$ for "M & H", $\tilde{T}_g = T/(\rho_p \dot{\gamma}^2 d^2)$ for "Bagnold, inertia", and $\tilde{T}_g = T/(\eta \dot{\gamma}^2)$ for "Bagnold, viscous", where $T$ is dispersive stress in Ref. [8]). It shows that our data for the granular temperature have similar scaling as that of dispersive stresses in Ref. [8], except when solid fraction is so large that the system is approaching a jamming state.

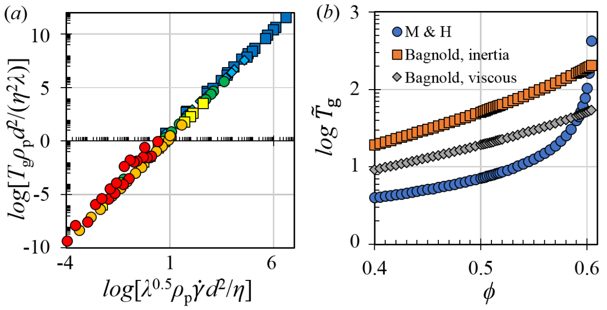


FIG. 3. (a) the relationship between $T_g \rho_p d^2/(\lambda \eta^2)$ and Bagnold number $Ba = \lambda^{0.5} \rho_p d^2 \dot{\gamma}/\eta$. (b) the relationship between normalized granular temperature or kinetic stress and the solid fraction. Here the relationship found in this letter is obtained by fitting FIG. 3(a) in the letter, and $\tilde{T}_g = T_g/(\rho_p d^2 \dot{\gamma}^2) \propto (\phi_m - \phi)^{-0.876}$. Also, $\tilde{T}_g = T/(\rho_p d^2 \dot{\gamma}^2) \propto \lambda^2$ for the grain inertia dominating cases, and $\tilde{T}_g = T/(\eta \dot{\gamma}) \propto \lambda^{1.5}$ for viscosity dominating cases, where $T$ is the dispersive stress in Ref. [8].

Our data of granular temperature show sudden change of scaling law between the granular temperature and the solid fraction, where $T_g$ increases with the increase of solid fraction when $\phi \gtrsim 0.51$, and $T_g$ decreases with the increase of solid fraction when $\phi \lesssim 0.51$. Based on the kinetic theory [9] of granular materials, Lun [10] and Campbell [11] found that normalized kinetic stresses scaled with the solid fraction of granular materials. As they in-

creased the solid fraction, the normalized kinetic stresses were also increased, which is similar to our results when solid fraction is approximately larger than 0.50 (FIG. 3(a)). Based on their calculation, when the solid fraction is very small, as they decreased the solid fraction, the kinetic stresses increased accordingly. This is similar to our sytsem results for the granular temperature (FIG. 3(a)), again, provided $\phi \gtrapprox 0.51$.


[1] P. Cundall and O. Strack, Géotechnique **29**, 47 (1979).
[2] Y. Tsuji, T. Tanaka, and T. Ishida, Powder Technol. **71**, 239 (1992).
[3] S. F. Foerster, M. Y. Louge, H. Chang, and K. Allia, Phys. Fluids **6**, 1108 (1994).
[4] O. Pitois, P. Moucheront, and X. Chateau, J. Colloid Interf. Sci. **231**, 26 (2000).
[5] A. Goldman, R. Cox, and H. Brenner, Chem. Eng. Sci. **22**, 653 (1967).
[6] P. Liu, R. Yang, and A. Yu, Chem. Eng. Sci. **86**, 99 (2013).
[7] J. S. Marshall and S. Li, *Adhesive particle flow* (Cambridge University Press, 2014).
[8] R. A. Bagnold, Proc. R. Soc. Lond. A **225**, 49 (1954).
[9] S. B. Savage and K. Hutter, J. Fluid Mech. **199**, 177 (1989).
[10] C. Lun, J. fluid Mech. **233**, 539 (1991).
[11] C. S. Campbell, Annu. Rev. Fluid Mech. **22**, 57 (1990).
