# Supplementary material for: Rheology of Thickly-Coated Granular-Fluid Systems
Source: arXiv:1812.07083 source file (2018-12-17)
Supplement: Supplementary file 2 [file supplemental_material_2.pdf]

# Rheology of Thickly-Coated Granular-Fluid Systems
# Supplemental Material II

Teng Man, Qingfeng Feng, Kimberly Hill

Table 1. Information of the inertia numbers in each simulation

| $\eta_f$ (cP) | $\sigma$ (Pa) | 100 | 100 | 100 | 100 | 100 | 100 | 200 | 200 | 500 | 500 |
|---|---|---|---|---|---|---|---|---|---|---|---|
| | $U_w$ (m/s) | 0.01 | 0.032 | 0.1 | 0.32 | 1.0 | 3.2 | 0.2 | 2.0 | 0.5 | 2.5 |
| 0.0 | $I_c$ | $2.5\times10^{-3}$ | $8.0\times10^{-3}$ | $2.5\times10^{-2}$ | $7.9\times10^{-2}$ | $2.5\times10^{-1}$ | $6.9\times10^{-1}$ | $3.5\times10^{-2}$ | $3.3\times10^{-1}$ | $5.6\times10^{-2}$ | $2.7\times10^{-1}$ |
| | $I_v$ | 0.0 | 0.0 | 0.0 | 0.0 | 0.0 | 0.0 | 0.0 | 0.0 | 0.0 | 0.0 |
| $2\times10^{-3.5}$ | $I_c$ | | | | | | $6.9\times10^{-1}$ | | | | |
| | $I_v$ | | | | | | $3.4\times10^{-7}$ | | | | |
| $2\times\ 10^{-3}$ | $I_c$ | | | | | $2.5\times10^{-1}$ | | | $3.3\times10^{-1}$ | | $2.7\times10^{-1}$ |
| | $I_v$ | | | | | $3.7\times10^{-7}$ | | | $3.6\times10^{-7}$ | | $1.8\times10^{-7}$ |
| $2\times10^{-2.5}$ | $I_c$ | | | | $7.9\times10^{-2}$ | | $6.9\times10^{-1}$ | | | | |
| | $I_v$ | | | | $3.9\times10^{-7}$ | | $3.4\times10^{-6}$ | | | | |
| $2\times10^{-2}$ | $I_c$ | | | $2.5\times10^{-2}$ | | $2.5\times10^{-1}$ | | $3.5\times10^{-2}$ | $3.3\times10^{-1}$ | $5.6\times10^{-2}$ | $2.7\times10^{-1}$ |
| | $I_v$ | | | $3.9\times10^{-7}$ | | $3.7\times10^{-6}$ | | $3.9\times10^{-7}$ | $3.6\times10^{-6}$ | $3.8\times10^{-7}$ | $1.8\times10^{-6}$ |
| $2\times10^{-1.5}$ | $I_c$ | | $8.0\times10^{-3}$ | | $7.9\times10^{-2}$ | | $6.9\times10^{-1}$ | | | | |
| | $I_v$ | | $3.9\times10^{-7}$ | | $3.9\times10^{-6}$ | | $3.4\times10^{-5}$ | | | | |
| $2\times10^{-1}$ | $I_c$ | $2.5\times10^{-3}$ | | $2.5\times10^{-2}$ | | $2.5\times10^{-1}$ | | $3.5\times10^{-2}$ | $3.3\times10^{-1}$ | $5.6\times10^{-2}$ | $2.7\times10^{-1}$ |
| | $I_v$ | $3.9\times10^{-7}$ | | $3.9\times10^{-6}$ | | $3.7\times10^{-5}$ | | $3.9\times10^{-6}$ | $3.6\times10^{-5}$ | $3.8\times10^{-6}$ | $1.8\times10^{-5}$ |
| $2\times10^{-0.5}$ | $I_c$ | | $8.0\times10^{-3}$ | | $7.9\times10^{-2}$ | | $6.9\times10^{-1}$ | | | | |
| | $I_v$ | | $3.9\times10^{-6}$ | | $3.9\times10^{-5}$ | | $3.4\times10^{-4}$ | | | | |
| $2\times10^{-0}$ | $I_c$ | $2.5\times10^{-3}$ | | $2.5\times10^{-2}$ | | $2.5\times10^{-1}$ | | $3.5\times10^{-2}$ | $3.3\times10^{-1}$ | $5.6\times10^{-2}$ | $2.7\times10^{-1}$ |
| | $I_v$ | $3.9\times10^{-6}$ | | $3.9\times10^{-5}$ | | $3.7\times10^{-4}$ | | $3.9\times10^{-5}$ | $3.6\times10^{-4}$ | $3.8\times10^{-5}$ | $1.8\times10^{-4}$ |
| $2\times10^{0.5}$ | $I_c$ | | $8.0\times10^{-3}$ | | $7.9\times10^{-2}$ | | $6.9\times10^{-1}$ | | | | |
| | $I_v$ | | $3.9\times10^{-5}$ | | $3.9\times10^{-4}$ | | $3.4\times10^{-3}$ | | | | |
| $2\times10^{1}$ | $I_c$ | $2.5\times10^{-3}$ | | $2.5\times10^{-2}$ | | $2.5\times10^{-1}$ | | $3.5\times10^{-2}$ | $3.3\times10^{-1}$ | $5.6\times10^{-2}$ | $2.7\times10^{-1}$ |
| | $I_v$ | $3.9\times10^{-5}$ | | $3.9\times10^{-4}$ | | $3.7\times10^{-3}$ | | $3.8\times10^{-4}$ | $3.6\times10^{-3}$ | $3.8\times10^{-4}$ | $1.8\times10^{-3}$ |

| | | | | | | | | | | | |
|---|---|---|---|---|---|---|---|---|---|---|---|
| $2\times10^{1.5}$ | $I_c$ | | $7.9\times10^{-3}$ | | $7.7\times10^{-2}$ | | $6.7\times10^{-1}$ | | | | |
| | $I_v$ | | $3.9\times10^{-4}$ | | $3.7\times10^{-3}$ | | $3.3\times10^{-2}$ | | | | |
| $2\times10^{2}$ | $I_c$ | $2.5\times10^{-3}$ | | $2.4\times10^{-2}$ | | $2.3\times10^{-1}$ | $6.3\times10^{-1}$ | $3.4\times10^{-2}$ | $3.1\times10^{-1}$ | $5.4\times10^{-2}$ | $2.6\times10^{-1}$ |
| | $I_v$ | $3.9\times10^{-4}$ | | $3.8\times10^{-3}$ | | $3.4\times10^{-2}$ | $1.0\times10^{-1}$ | $3.7\times10^{-3}$ | $3.4\times10^{-2}$ | $3.8\times10^{-3}$ | $1.8\times10^{-2}$ |
| $1.33\times10^{2}$ | $I_c$ | | | | | | | | | | $2.3\times10^{-1}$ |
| | $I_v$ | | | | | | | | | | $1.0\times10^{-1}$ |
| $2\times10^{2.5}$ | $I_c$ | | $7.7\times10^{-3}$ | | $7.1\times10^{-2}$ | $2.1\times10^{-1}$ | $5.6\times10^{-1}$ | | $2.9\times10^{-1}$ | | |
| | $I_v$ | | $3.7\times10^{-3}$ | | $3.5\times10^{-2}$ | $1.0\times10^{-1}$ | $2.7\times10^{-1}$ | | $1.0\times10^{-1}$ | | |
| $2\times10^{3}$ | $I_c$ | $2.4\times10^{-3}$ | $7.5\times10^{-3}$ | $2.3\times10^{-2}$ | $6.5\times10^{-2}$ | $1.8\times10^{-1}$ | $4.8\times10^{-1}$ | $3.2\times10^{-2}$ | $2.5\times10^{-1}$ | $5.0\times10^{-2}$ | $2.2\times10^{-1}$ |
| | $I_v$ | $3.8\times10^{-3}$ | $1.1\times10^{-2}$ | $3.5\times10^{-2}$ | $1.0\times10^{-1}$ | $2.8\times10^{-1}$ | $7.4\times10^{-1}$ | $3.5\times10^{-2}$ | $2.8\times10^{-1}$ | $3.5\times10^{-2}$ | $1.5\times10^{-1}$ |
| $2\times10^{3.5}$ | $I_c$ | $2.4\times10^{-3}$ | $7.1\times10^{-3}$ | $2.1\times10^{-2}$ | $5.7\times10^{-2}$ | $1.6\times10^{-1}$ | | $2.9\times10^{-2}$ | $2.2\times10^{-1}$ | $4.6\times10^{-2}$ | $1.9\times10^{-1}$ |
| | $I_v$ | $1.1\times10^{-2}$ | $3.5\times10^{-2}$ | $1.0\times10^{-1}$ | $2.8\times10^{-1}$ | $7.5\times10^{-1}$ | | $1.0\times10^{-1}$ | $7.4\times10^{-1}$ | $1.0\times10^{-1}$ | $4.1\times10^{-1}$ |
| $2\times10^{4}$ | $I_c$ | $2.2\times10^{-3}$ | $3.5\times10^{-2}$ | $1.8\times10^{-2}$ | | | | $2.5\times10^{-2}$ | | $4.0\times10^{-2}$ | |
| | $I_v$ | $3.5\times10^{-2}$ | $1.0\times10^{-1}$ | $2.8\times10^{-1}$ | | | | $2.8\times10^{-1}$ | | $2.8\times10^{-1}$ | |
| $2\times10^{4.5}$ | $I_c$ | $2.1\times10^{-3}$ | $5.8\times10^{-3}$ | | | | | | | | |
| | $I_v$ | $1.0\times10^{-1}$ | $2.8\times10^{-1}$ | | | | | | | | |
